# Supplementary material for: Verified Parameterized Choreographies Technical Report
Source: arXiv:2502.15382 source file (2025-04-15)
Supplement: Supplementary file 1 [file todos.tex]

\bnote{Say something about: participants in condition limits occurrence of endpoints in communicates, endpoint statements. Either 1) we severly restrict it in the semi-formal development, like in the first veymont tool paper, and we mention in the impl section that it can be done more leniently, or 2) the transformation needs to describe it. As I think it will result in some tricky proof obligations, probably 1) is better for now. Then this assumption needs to be documented.}
 
\bnote{Mention that symmetric version where the receiving side is a range omitted for brevity. Or just generality only supported by implementation. ``See implementation section''}

\bnote{TODO: Document typical elements that do not match the grammar, e.g. $E_l$ and $E_h$, use of $i$ for tid/index in endpoint family, etc.}
